# Supplementary material for: An Intermediate Representation for Composable Typed Streaming Dataflow Designs
Source: arXiv:2308.13436 source file (2023-09-28)
Supplement: Supplementary file 1 [file tilex.tex]

\begin{lstlisting}[basicstyle=\ttfamily\scriptsize,caption={TIL Example},label={lst:tilex}]
namespace my::example::space {
    // Type declarations
    type byte = Bits(8);
    // Type expressions can be identifers or in-line declarations
    type select = Union(val: byte, empty: Null);
    type rgb = Group(r: select, g: select, b: select);
    // Streams have many properties, but some are optional
    type stream = Stream (
        data: rgb,
        throughput: 2.0, // 1.0 by default
        dimensionality: 0,
        synchronicity: Sync,
        complexity: 4,
        direction: Forward, // Forward by default
        user: Null, // Null by default
        keep: false, // false by default
    );
    type stream2 = stream;

    // A streamlet declaration
    #documentation (optional)#
    streamlet comp1 = (
        // Ports are *name* : *direction* *stream expression*
        a: in stream,
        b: out stream,
        # port documentation #
        c: in stream2,
        d: out stream2,
    );

    // An independent interface declaration
    interface iface1 = (a: in stream, b: out stream);

    #streamlet documentation
newline documentation#
    streamlet comp2 = iface1;
    
    // Implementation declarations
    #This is implementation documentation.#
    impl struct = (
        a: in stream,
        b: out stream,
        c: in stream2,
        d: out stream2,
    ){
        // Ports can be connected with --
        a -- b;

        // Streamlet instances are declared with
        // *instance name* = *streamlet name*
        a = comp1;
        b = comp1;

        // Ports on streamlet instances can be addressed with .
        a.a -- b.b;
        a.b -- b.a;
        
        // Ports on instances can also be connected to local ports
        c -- a.c;
        d -- b.d;
        a.d -- b.c;
    };

    // Linked implementations are paths enclosed by double quotes.
    impl link = comp1 "./a/path/to/a/directory";

    streamlet comp3 = comp1 {
        impl:
        #This is implementation documentation, too.#
        {
            p1 = comp2;
            p2 = comp2;
            a -- p1.a;
            b -- p1.b;
            c -- p2.a;
            d -- p2.b;
        }
    };

    streamlet comp4 = comp1 { impl: struct };

    streamlet comp5 = comp1 { impl: "./a/path/to/a/directory" };
}
\end{lstlisting}
