# Supplementary material for: An Intermediate Representation for Composable Typed Streaming Dataflow Designs
Source: arXiv:2308.13436 source file (2023-09-28)
Supplement: Supplementary file 2 [file appendix.tex]

%%
%% If your work has an appendix, this is the place to put it.
\appendix

\section{Tydi Intermediate Language Examples}\label{app:til}

\todo{Include these snippets instead, point towards the repository for a full example file.}

% \lstinline{#documentation#}

%\includegraphics[width=0.7\linewidth]{snippets/typedecl.pdf}

%\includegraphics[width=0.8\linewidth]{snippets/ifacedecl.pdf}

% Alternative, in case I finish the parser in time
%\includegraphics[width=0.9\linewidth]{snippets/ifacedecldomains.pdf}

%\includegraphics[width=0.8\linewidth]{snippets/impldecl.pdf}

% Alternative, in case I finish the parser in time
%\includegraphics[width=0.9\linewidth]{snippets/impldecldomains.pdf}

%\includegraphics[width=0.85\linewidth]{snippets/streamletdecl.pdf}

%\input{sections/90_appendix/tilex}

%\todo{Example of the (proposed) test grammar?}

% \todo{Include this listing in the section directly?}

% \begin{lstlisting}[basicstyle=\ttfamily\scriptsize,caption={Proposed testing syntax},label={lst:testex}]
% test multiple_streams {
%     // Instantiate a Streamlet as the test subject
%     a = streamlet1;
%     // Equality automatically determines whether to drive
%     // or compare a transfer.
%     a.port_inout = {
%         in_field: "11",  // Acts
%         out_field: "11", // Asserts
%     };
%     // A sequence for a Stream with dimensionality=1
%     a.dim_seq = ["11", "00"];
%     // Independent transfers for a Stream with dimensionality=0 
%     a.flat_seq = ("11", "00");
% }

% test counter {
%     a = counter_streamlet;
%     // Sequences are useful for components with stateful logic
%     sequence "optional sequence name" {
%         // Names for stages and sequences are optional, but helpful
%         "initial state" {
%             a.count = "0000";
%         },
%         "add 1" {
%             a.inc = "01";
%         },
%         "result 1" {
%             a.count = "0001";
%         },
%         "add 0" {
%             a.inc = "00";
%         },
%         "result 2" {
%             a.count = "0001";
%         }
%         "add 1 again" {
%             a.inc = "01";
%         },
%         "result 3" {
%             a.count = "0010";
%         },
%     };
% }
% \end{lstlisting}
